# Supplementary material for: Consistent cosmic shear in the face of systematics: a B-mode analysis of KiDS-450, DES-SV and CFHTLenS
Source: arXiv:1810.02353 source file (2019-03-27)
Supplement: Supplementary file 1 [file AppendixA.tex]

The COSEBIs formalism introduced in \citep{SEK10} is written assuming a flat-sky approximation. Given then future surveys will 
probe very large scale and will reach almost the full extent of the sky, it is useful to be able to increase the angular range within which the COSEBIs are defined. The flat-sky approximation deviates from the truth (curved sky) as we try to probe larger angular distances. We can always limit the  maximum angular distance, $\theta_{\rm max}$ in our COSEBIs analysis to make sure this deviation is within the error budget of our survey. However in the next generation of surveys the error budget is small and also some valuable information can be gained by going to larger angular scales. Therefore, here we extend the COSEBIs formalism to the curved sky.

The 2PCFs for a curved sky are related to the shear power spectra by,
\begin{equation}
\label{eq:2PCFsCurved}
\xi_+(\theta)=\sum_{\ell=2}^\infty \frac{2\ell+1}{4\pi} C_\ell^\gamma d_{22}^\ell(\theta)~~~~~~~~ {\rm and}~~~~~~~~~\xi_-(\theta)=\sum_{\ell=2}^\infty \frac{2\ell+1}{4\pi} C_\ell^\gamma d_{2\;-2}^\ell(\theta)\;,
\end{equation}
where $C_\ell^\gamma$ is the shear power spectrum and is related to the convergence power spectrum through
\begin{equation}
C_\ell^{\kappa}=\frac{\ell(\ell+1)}{(\ell-1)(\ell+2)}C_\ell^\gamma\;,
\end{equation}
and $d_{mm'}^\ell(\theta)$ are elements of a Wigner (small) d-matrix \citep[see][]{Kilbinger17}. $C_\ell^{\kappa}$ can be written as the sum of E and B-mode power spectra, hence we can write,
\begin{equation}
C_\ell^\gamma=\frac{(\ell-1)(\ell+2)}{\ell(\ell+1)}(C_\ell^{\rm \kappa_E}+C_\ell^{\rm \kappa_B})\equiv C_\ell^{\rm \gamma_E}+C_\ell^{\rm \gamma_B}\;,
\end{equation}
where we defined E/B-mode shear power spectra for simplicity. As a first ansatz we write the COSEBIs E/B-modes as,
\begin{equation}
\label{eq:EBCurved1}
E(B)=\frac{1}{2}\int_{\theta_{\rm min}}^{\theta_{\rm max}}\d\vartheta \sin(\vartheta)[\xi_+(\vartheta)T_{+}(\vartheta)\pm\xi_-(\vartheta)T_-(\vartheta)]\;,
\end{equation}
where we replaced a $\theta$ in Eqs.\thinspace\eqref{eq:EnReal} and \eqref{eq:BnReal} with $\sin(\theta)$ 
and dropped the redshift bin indices. Replacing $\xi_\pm$ from \Eqt\eqref{eq:2PCFCurved} into \Eqt\eqref{eq:EBCurved1} we reach,
\begin{equation}
\label{eq:EBCurved2}
E(B)=\sum_{\ell=2}^\infty \frac{2\ell+1}{4\pi} \left\lbrace C_\ell^{\rm \gamma_E}[W_+^\ell\pm W_-^\ell]+ C_\ell^{\rm \gamma_B}[W_+^\ell \mp W_-^\ell]\right\rbrace\;,
\end{equation}
with
\begin{equation}
W_+^\ell=\frac{1}{2}\int_0^\infty \d\theta\sin(\theta)T_+(\theta)d^\ell_{2\;2}(\theta)~~~~~~~~~~ and ~~~~~~~~~ W_-^\ell=\frac{1}{2}\int_0^\infty \d\theta\sin(\theta)T_-(\theta)d^\ell_{2\;-2}(\theta)\;.
\end{equation}
For E and B in \Eqt\eqref{eq:EBCurved2} to only depend on their corresponding power spectrum we need $W_+^\ell=W_-\ell$, which result in the following condition,
\begin{equation}
\label{eq:Tpm}
\int_0^\infty \d\theta\sin(\theta)T_+(\theta)d^\ell_{2\;2}(\theta)=\int_0^\infty \d\theta\sin(\theta)T_-(\theta)d^\ell_{2\;-2}(\theta)\;. 
\end{equation}
\cite{SchneiderKilbinger07} found relations between $T_\pm(\theta)$ that ensure pure E/B-modes. 
Here we follow those steps for a curved sky. Note that for $\ell>>2$ $d^\ell_{2\;2}(\theta)\approx J_0(\ell\theta)$ and 
$d^\ell_{2\;2}(\theta)\approx J_4(\ell\theta)$, and $\sin(\theta)\approx\theta$ for small angles. These approximations are done for a flat-sky which holds for angular ranges much smaller than the full-sky. 

Wigner d-matrices form a complete and orthogonal set of functions. The completeness relation for $d^\ell_{mm'}(\theta)$ is given
 by
 \begin{equation}
 \label{eq:completeness}
 \sum_{\ell={\rm max[|m|,|m'|]}}^{\infty} \frac{2\ell+1}{2} d^\ell_{mm'}(\theta) d^\ell_{mm'}(\theta') =\delta_{\rm D}(\cos\theta-\cos\theta')\;,
 \end{equation}
where $\delta_{\rm D}$ is the Dirac delta function \citep[see][for example]{Chon04}. The $d^\ell_{mm'}(\theta)$ also follow several recursive relations. We use the following two in our calculations,
\begin{equation}
d
\end{equation}
and 
\begin{equation}
d
\end{equation}
Using the above equation we can find two relations between $T_\pm$. Firstly we multiple \Eqt\eqref{eq:Tpm} by $\sum_{\ell={\rm max[|m|,|m'|]}}^{\infty} \frac{2\ell+1}{2} d^\ell_{2\;2}(\theta)$ and find
\begin{equation}
T_+=T_-
\end{equation}
Then we do the same with $d^\ell_{2\;-2}(\theta)$ and find
\begin{equation}
T_-(\theta)=T_+(\theta)+\frac{1}{\sin^2(\frac{\theta}{2})}\int_0^\theta\d\vartheta\sin\vartheta T_+(\vartheta) \sec^4(\vartheta/2)-\frac{2(2+\cos\theta)}{\sin^4(\frac{\theta}{2})}\int_0^\theta\d\vartheta T_+(\vartheta)\tan^3\frac{\vartheta}{2}
\end{equation}
Note that for the small angle limit these equations will simplify to 
\begin{equation}
T_+=T_-
\end{equation}
which where derived in \cite{SchneiderKilbinger07}.
